# Supplementary material for: MultiNeRF: Multiple Watermark Embedding for Neural Radiance Fields
Source: arXiv:2504.02517 source file (2025-04-03)
Supplement: Supplementary file 1 [file supplementary.tex]

\clearpage
\appendix
\twocolumn[{%
    \centering
    {\Large \textbf{MultiNeRF: Multiple Watermark Embedding for Neural Radiance Fields}} \\[1em]
    {\Large Supplementary Material} \\[2em]
}]

\section*{A. Training HiDDeN Decoder}
\label{sec:supp_impl_details}
\begin{figure*}[t]
    \centering
    \includegraphics[width=\textwidth]{ICCV2025-Author-Kit-Feb/hidden_decoder.png}
    \caption{HiDDeN decoder}
    \label{fig:hidden_decoder_image}
\end{figure*}

\begin{figure*}[t]
    \centering
    \includegraphics[width=0.8\textwidth]{ICCV2025-Author-Kit-Feb/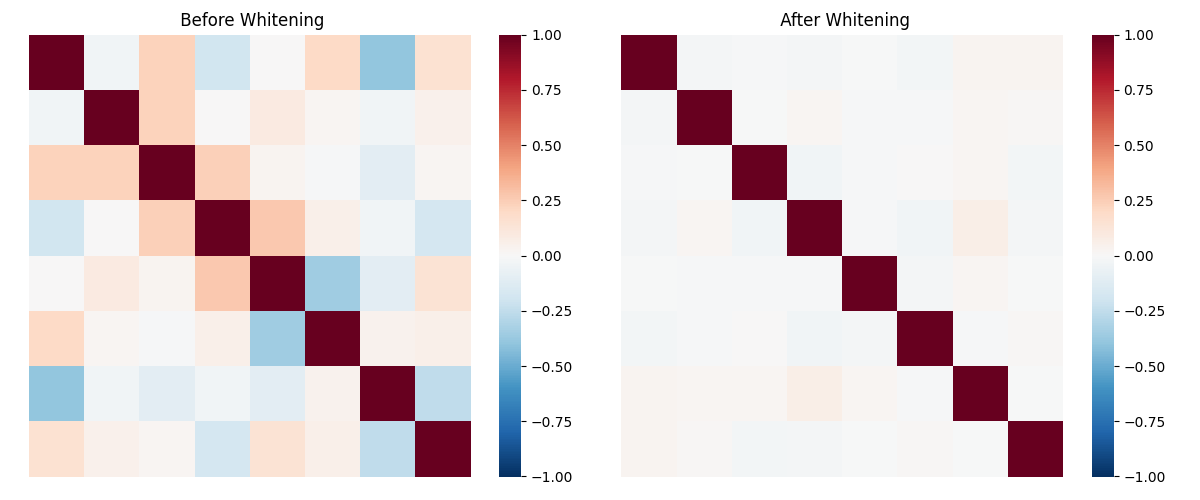}
    \caption{Covariance Matrix of the bit outputs before and after whitening}
    \label{fig:covariance}
\end{figure*}

\begin{figure*}[t]
    \centering
    \includegraphics[width=0.8\textwidth]{ICCV2025-Author-Kit-Feb/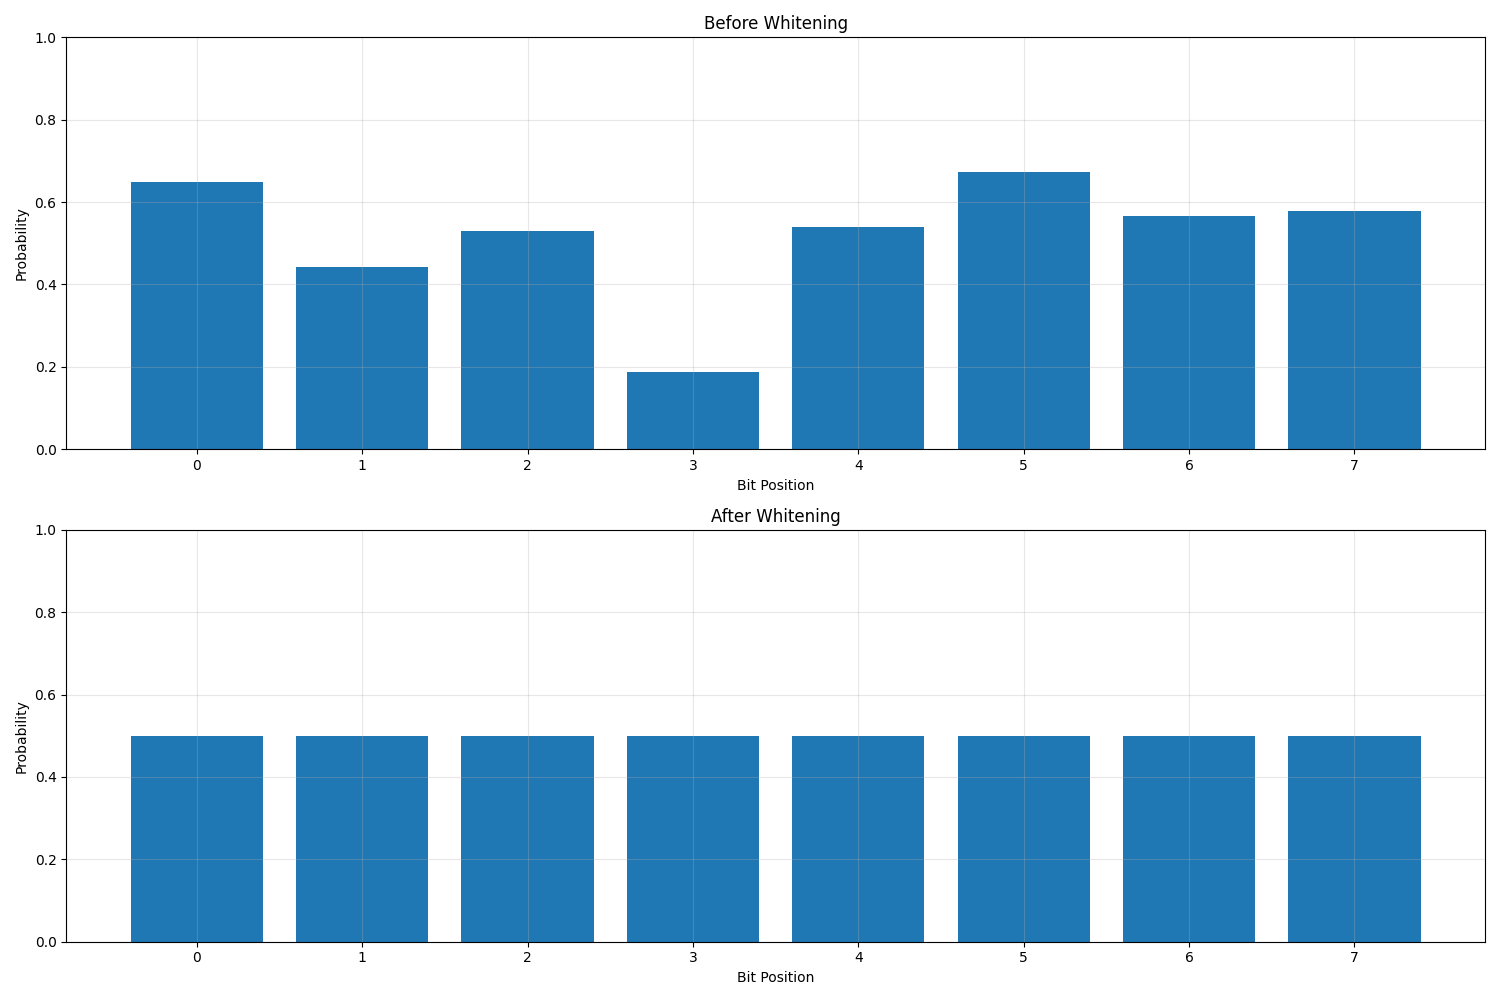}
    \caption{Probability of bit outputs from decoder before and after whitening}
    \label{fig:probability}
\end{figure*}

\noindent \textbf{Training.} To enable robust message extraction from the rendered images, we adopt a standard deep watermarking approach HiDDeN \cite{zhu2018hidden}, we use the training code from \cite{fernandez2023stable} to train the HiDDeN decoder. \cref{fig:hidden_decoder_image} shows the training of HiDDeN, where the encoder takes a cover image and a binary message to watermark, then outputs a watermarked image. A noise layer simulates common distortions (e.g., cropping, JPEG compression, rotation). The decoder then attempts to recover the embedded bits from the distorted watermarked image.

Because our main pipeline only requires the decoder, once training converges, we discard the encoder entirely and keep only the decoder.

\noindent \textbf{Optimization.} We train the decoder on MS-COCO 2014 dataset \cite{lin2014microsoft} keeping the image resolution at 256 x 256. The optimization is carried out on 4 GPUs, with Lamb optimizer \cite{you2019large}. The batch size is kept at 16, while the learning rate is $5e-3$

\noindent \textbf{Whitening.} We observe that the outputs could be biased or correlated when the trained decoder is exposed to non-watermarked images later. To address this, we apply PCA-whitening to the linear layer of the decoder, similar to \cite{fernandez2023stable}. This step de-correlates the output bits and helps eliminate systematic biases (as shown in \cref{fig:covariance} \& \cref{fig:probability}), ensuring the decoder provides more reliable and unbiased watermark predictions in our method.

\section*{B. Differentiable Augmentation Layer.}
\label{sec:supp_results}
We introduce a differentiable augmentation layer to strengthen our watermark decoder's robustness against image degradations. During training, the rendered image is randomly subjected to one or more lightweight augmentations (e.g., blur, JPEG compression, color jitter). The augmented image is then fed into the watermark decoder. Because these augmentations are implemented with differentiable operations (via Kornia \cite{riba2020kornia} and the differentiable JPEG compression implementation comes from \cite{shin2017jpeg}), the decoder can learn to handle distortions in an end-to-end fashion.

This is how the augmentation is organized:

\noindent \textbf{1.Augmentation Pool.} We maintain a set $\{ A_1, A_2, \dots, A_m \}$ of possible transformations, such as random blur, random noise, or random brightness. Each augmentation is parameterized by a probability $p = 0.75$ that determines whether it is applied.

\noindent \textbf{2. Random Selection.} At every training step, we randomly select 2 augmentations from the pool and apply them sequentially. As a result, each image may be subjected to different combinations of distortions, making the model more robust.

\cref{tab:low_severity_aug_params} lists the parameter ranges for each augmentation used in training the model. \cref{fig:different_augmentation_examples} shows the visual examples of each augmentation. 

\begin{table}[h]
\centering
\resizebox{\columnwidth}{!}{%
\begin{tabular}{l l}
\toprule
\textbf{Transformation} & \textbf{Parameter(s)} \\
\midrule
JPEG Quality        & 30 \\
Brightness          & (0.9, 1.1) \\
Contrast            & (0.9, 1.1) \\
Color Jitter        & (0.05, 0.05, 0.05, 0.01) \\
Gaussian Blur       & Kernel: (3, 3); Sigma: (0.1, 1.0) \\
Gaussian Noise      & Std: 0.02 \\
Hue                 & $\pm$0.01 \\
Posterize           & 5 bits \\
RGB Shift           & Shift limit: 0.02 \\
Saturation          & (0.9, 1.1) \\
Median Blur         & Kernel: (3, 3) \\
Box Blur            & Kernel: (3, 3) \\
Motion Blur         & Kernel: (3, 5); Angle: $\pm$25$^\circ$; Direction: $\pm$0.25 \\
Sharpness           & 0.5 \\
\bottomrule

\end{tabular}%
}
\caption{Augmentation Parameters while training MultiNeRF}
\label{tab:low_severity_aug_params}
\end{table}

\begin{figure*}[t]
    \centering
    \includegraphics[width=\textwidth]{ICCV2025-Author-Kit-Feb/supp_augmentation.png}
    \caption{Examples of different augmentations applied during training}
    \label{fig:different_augmentation_examples}
\end{figure*}

\section*{C. Additional Details on the User Study}
\label{sec:user_study_supple}
We conducted our user study on Amazon Mechanical Turk (MTurk), recruiting six unique participants. Each participant was presented with 180 image pairs in randomized order. In each pair, one image was the ground-truth image, and the other was the watermarked image output produced by one of the watermarking methods (e.g., MultiNeRF, WateRF, WateRF-modified, or NeRFProtector). 

The participants were asked to “Compare the Ground-Truth (GT) image and the AI-processed image. and Does the processed image have blotches or color/rainbow artifacts compared to the GT image?” They then rated the overall severity of any artifacts on a five-point scale (\cref{tab:artifact_severity}).

\begin{table}[h]
    \centering
    \small
    \begin{tabular}{|c|l|}
        \hline
        \textbf{Rating} & \textbf{Description} \\ 
        \hline
        5 & Severe artifacts that significantly impact image quality \\ 
        \hline
        4 & Clearly visible artifacts \\ 
        \hline
        3 & Some visible artifacts upon closer inspection \\ 
        \hline
        2 & Barely noticeable artifacts \\ 
        \hline
        1 & No visible artifacts \\ 
        \hline
    \end{tabular}
    \caption{Severity scale for AI-processed image artifacts}
    \label{tab:artifact_severity}
\end{table}

\begin{figure*}[t]
    \centering
    \includegraphics[width=0.9\textwidth]{ICCV2025-Author-Kit-Feb/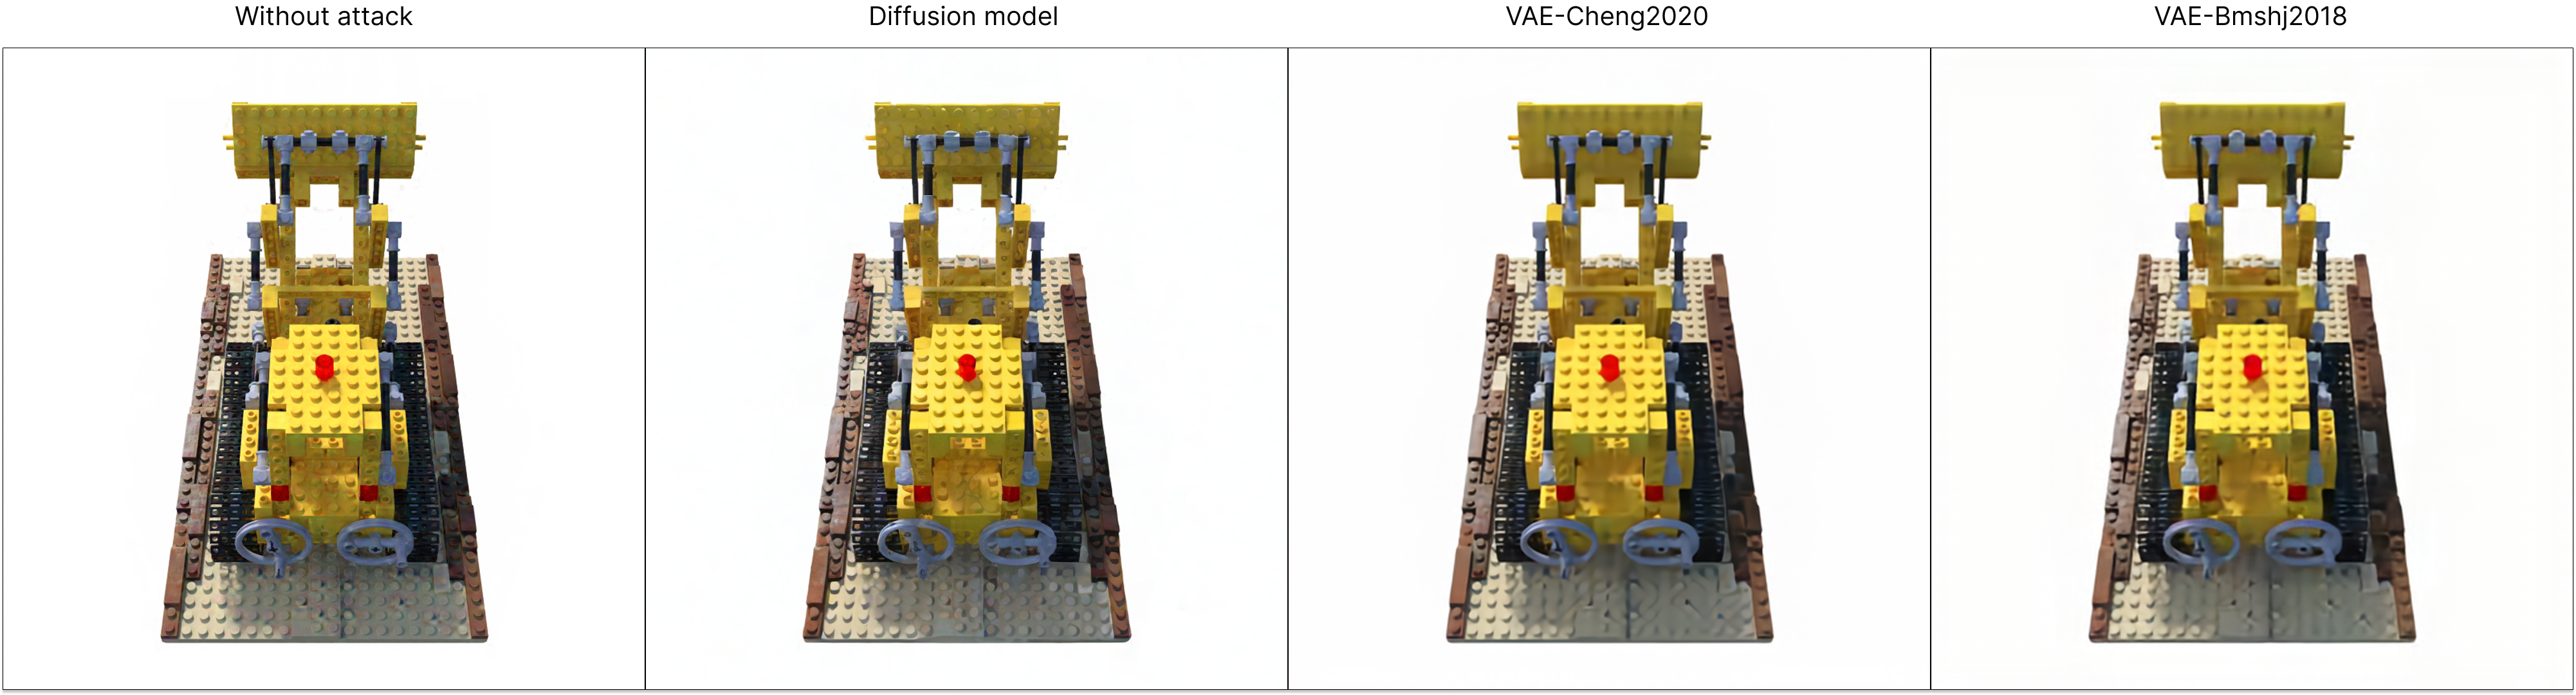}
    \caption{Regeneration attacks}
    \label{fig:regeneration_attack_examples}
\end{figure*}

\begin{figure*}[t]
    \centering
    \includegraphics[width=0.6\textwidth]{ICCV2025-Author-Kit-Feb/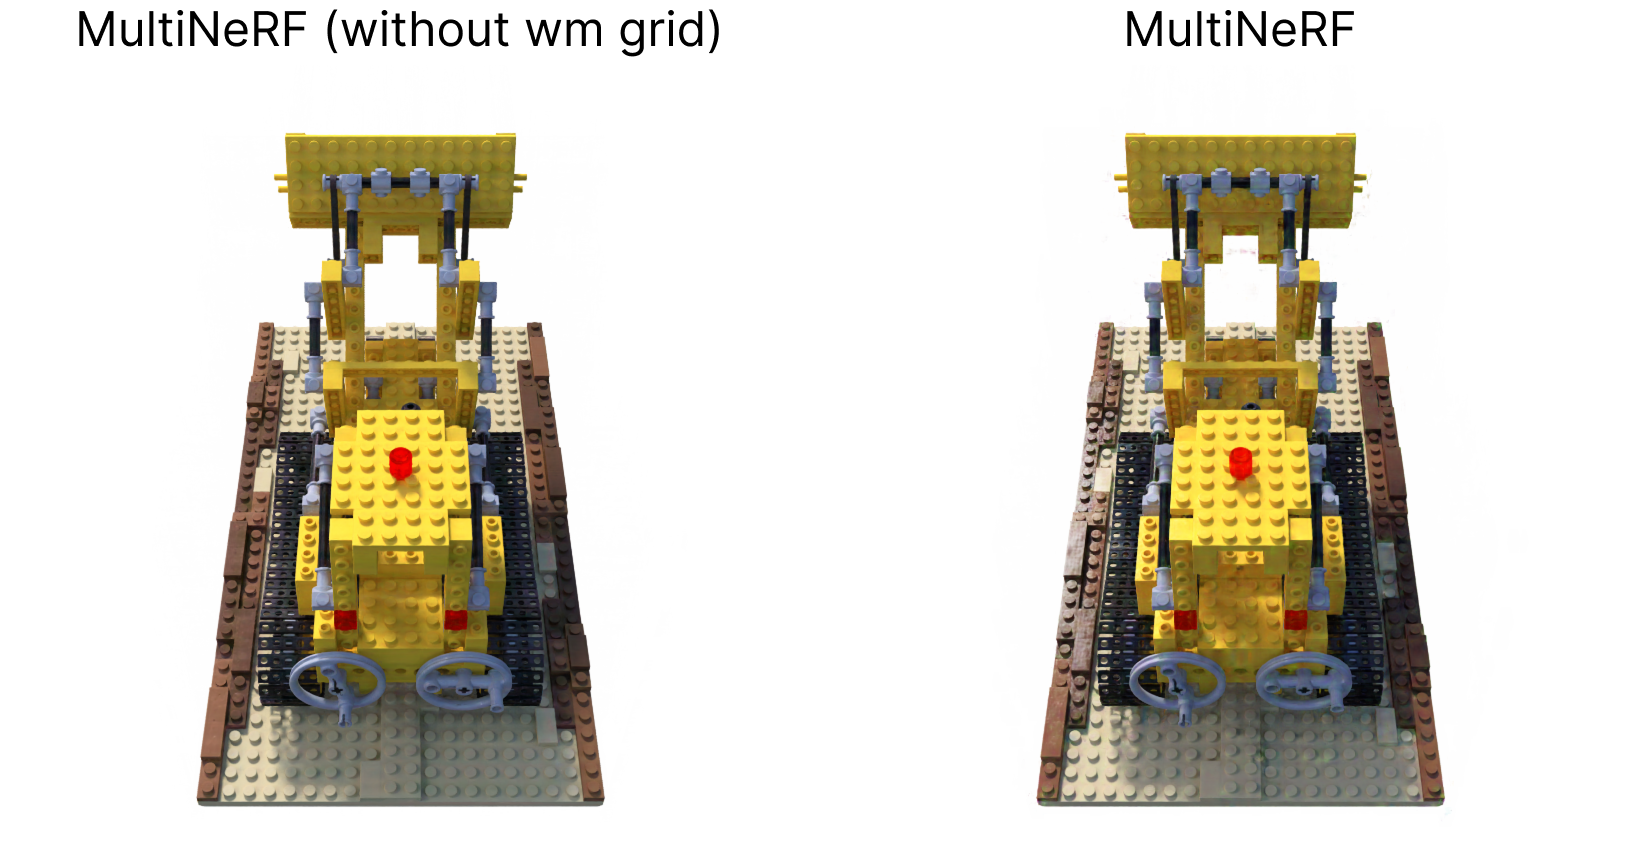}
    \caption{MultiNeRF (without watermark grid) vs MultiNeRF (Full method) image quality. Without the grid, we see that we mostly lose reflection information.}
    \label{fig:without_grid_compare}
\end{figure*}

\begin{figure*}[t]
    \centering
    \includegraphics[width=0.9\textwidth]{ICCV2025-Author-Kit-Feb/user_study.png}
    \caption{Examples of the images used for user study}
    \label{fig:user_study_image_examples}
\end{figure*}

\begin{figure*}[t]
    \centering
    \includegraphics[width=\textwidth]{ICCV2025-Author-Kit-Feb/extra_results.png}
    \caption{MultiNeRF results on the other synthetic and LLFF dataset}
    \label{fig:extra_results}
\end{figure*}
